# Supplementary material for: Higgs and non-universal gaugino masses: no SUSY signal expected yet?
Source: arXiv:1202.5288 ancillary file (2012-05-30)
Supplement: Supplementary file 1 [file logprior.pdf]

## Supplement to: Higgs and non-universal gaugino masses: no SUSY signal expected yet?

---

**Sascha Caron,<sup>a,b</sup> Jari Laamanen,<sup>a,b</sup> Irene Niessen<sup>a,b</sup> Antonia Strübig<sup>c</sup>**

<sup>a</sup>*Experimental and Theoretical High Energy Physics, IMAPP, Faculty of Science, Radboud University Nijmegen, Mailbox 79, P.O. Box 9010, NL-6500 GL Nijmegen, The Netherlands*

<sup>b</sup>*Nikhef, Science Park 105, 1098 XG Amsterdam, The Netherlands*

<sup>c</sup>*Physikalisches Institut, University of Freiburg, Hermann-Herder Str.3, 79104 Freiburg, Germany*

*E-mail:* [Sascha.Caron@cern.ch](mailto:Sascha.Caron@cern.ch), [j.laamanen@science.ru.nl](mailto:j.laamanen@science.ru.nl),  
[i.niessen@science.ru.nl](mailto:i.niessen@science.ru.nl), [antonia.struebig@cern.ch](mailto:antonia.struebig@cern.ch)

**ABSTRACT:** So far, no supersymmetric particles have been detected at the Large Hadron Collider (LHC). However, the recent Higgs results has interesting implications for the SUSY parameter space. In this paper, we study the consequences of an LHC Higgs signal for a model with non-universal gaugino masses in the context of SU(5) unification. The gaugino mass ratios associated with the higher representations produce viable spectra that are largely inaccessible to the current LHC and direct dark matter detection experiments. Thus, in light of the Higgs results, the non-observation of SUSY is no surprise.

**KEYWORDS:** Supersymmetry, Grand Unified Theory, Higgs, Dark Matter

## A Results for Logarithmic Prior

In this supplement, we show the plots for the logarithmic prior. The ranges of this prior are the same as those for the flat prior, but the variables  $m_0$  and  $M_3$  are distributed logarithmically.

Figure A.1 shows the results for the stop masses. We see some minor changes because the logarithmic prior emphasizes the low mass range, but the main conclusions remain unchanged: not both stops can be light, but the lightest stop can be considerably lighter than 1 TeV due to mixing.

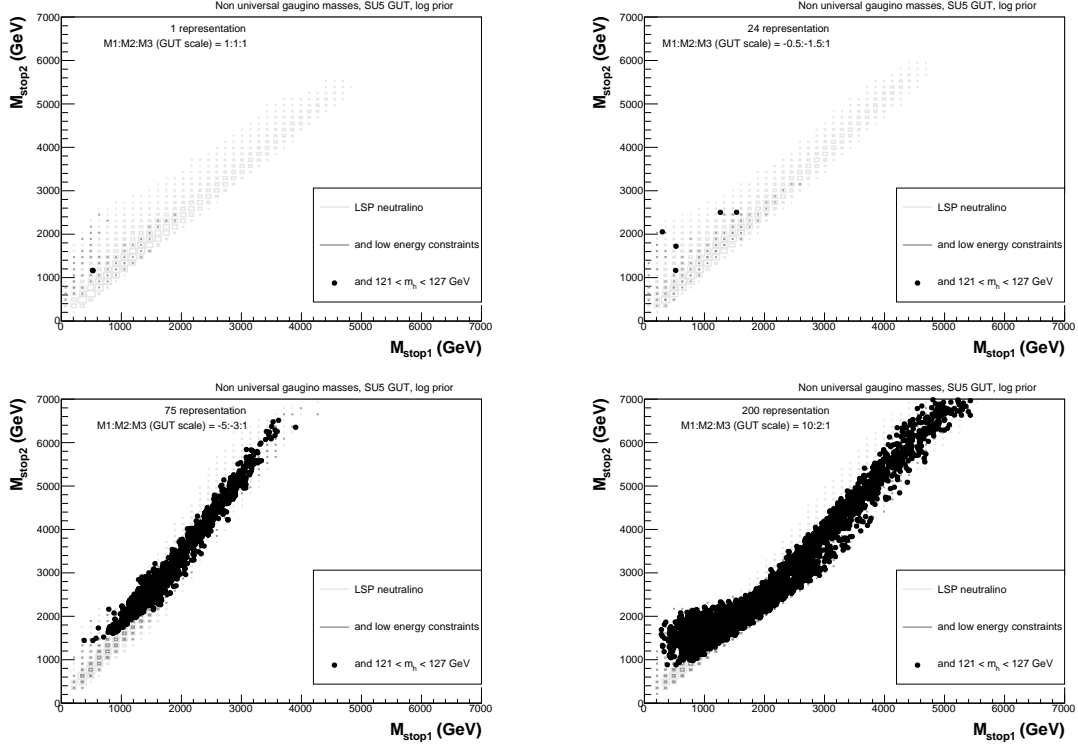

Figure A.1. Stop masses in the different representations for the log prior.

Figure A.2 shows the squark-gluino mass plane. We see once again that light light-flavoured squarks are excluded, but that light gluinos are still a viable option.

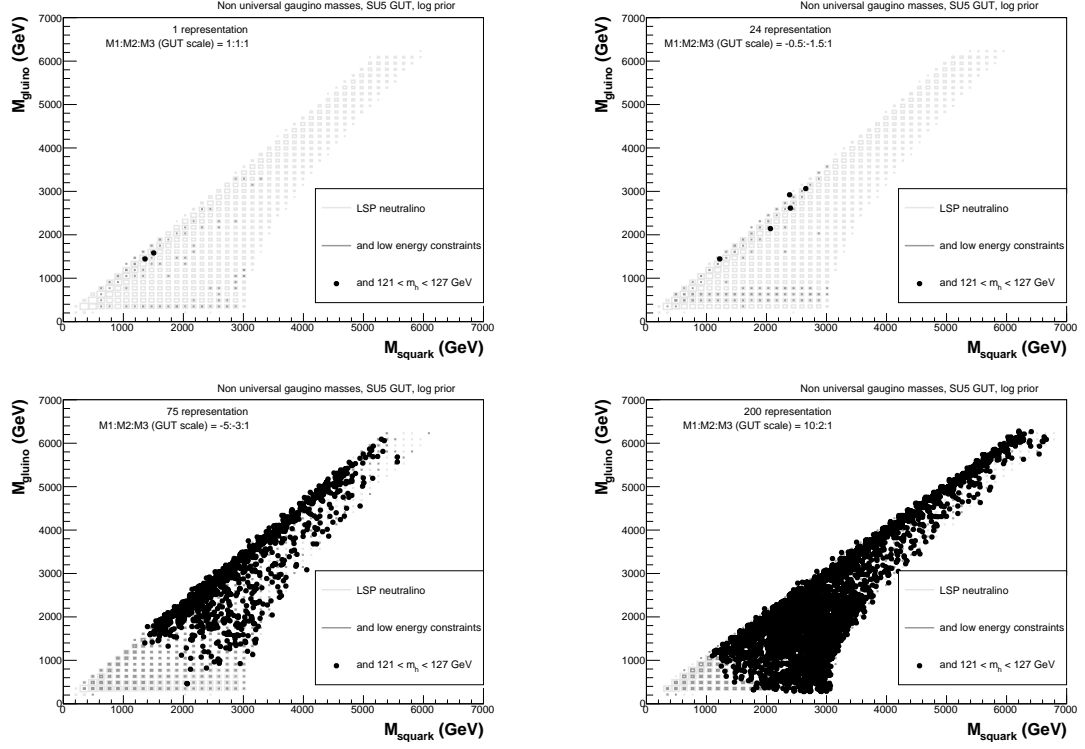

**Figure A.2.** Squark and gluino masses in the different representations for the log prior.
